# Supplementary material for: Fair Bayesian Optimization
Source: arXiv:2006.05109 source file (2021-06-18)
Supplement: Supplementary file 1 [file appendix_representation.tex]

\section{Fair Representation}
We can define $h: \mathcal{D} \rightarrow \mathcal{D}'$ (where $\mathcal{D}$ and $\mathcal{D}'$ can be seen as $\mathbb{R}^d$) as a function that changes the representation of the examples. It can be in general a parametric preprocessing method of the data (e.g., a neural network that learns a representation).

In the following, our current pipeline:%
\begin{align}
\begin{bmatrix} \xb \\ \mathcal{D} \end{bmatrix} &\rightarrow A(\xb, \mathcal{D}) \rightarrow M \rightarrow \begin{bmatrix} \text{loss}_{\mathcal{D}}(M) \\ \text{bias}_{\mathcal{D}}(M) \end{bmatrix}, %
\end{align}
where $A$ is a learning algorithm that, given $\xb$ and a dataset $\mathcal{D}$, produces a predictive model $M$. Then, we are able to evaluate the loss and bias of $M$ over $\mathcal{D}$.

Fair BO learns a surrogate model $f$ such that: \begin{equation}
    f(\xb, \mathcal{D}) \approx \begin{bmatrix} \text{loss}_{\mathcal{D}}(M) \\ \text{bias}_{\mathcal{D}}(M) \end{bmatrix}.
\end{equation}

We are now interested in changing our pipeline adding the new representation $h$. In this sense, the final opaque method that Fair BO will have to optimize in a \blackbox manner would automatically include the function $h$ on top, i.e.,
\begin{align}
\xb \rightarrow A(\xb,h(\mathcal{D})) \rightarrow M \rightarrow \begin{bmatrix} \text{loss}_{h(\mathcal{D})}(M) \\ \text{bias}_{h(\mathcal{D})}(M) \end{bmatrix}.
\end{align}
Consequently, fair BO should be able to provide an $f$ such that: \begin{equation}
    f(\xb, \mathcal{D}) \approx \begin{bmatrix} \text{loss}_{h(\mathcal{D})}(M) \\ \text{bias}_{h(\mathcal{D})}(M) \end{bmatrix}.
\end{equation}

The issue here is to optimize the parameters of the representation function $h$. This task would be straightforward knowing the gradient of the opaque function. Using the same BO process to optimize all the parameters of $h$ is computationally not feasible considering that $h$ has to be sufficiently expressive, and thus it needs more than few dozens of parameters. Additionally, standard Gaussian-process based BO struggles in such a large hyperparameter regime.

Given a trained model $M$ we need to be able to create a model that distills or mimics $M$, in the sense of its gradient (and not its output), w.r.t. the input. This is not very common in the literature where most distillation methods try to have a simpler (or faster) model that mimics the input-output behavior of the original one (usually in a teacher-student fashion, where the teacher is not even an opaque function).

In other words, we need a function $d$ s.t.
\begin{equation}
    d(\mathcal{D}) \approx \nabla_\mathcal{D} \begin{bmatrix} \text{loss}_{\mathcal{D}}(M) \\ \text{bias}_{\mathcal{D}}(M) \end{bmatrix},
\end{equation}
where $M$ is a trained opaque model.  A graphical example in Figure~\ref{fig:idea}.
\begin{figure*}
\centering
\begin{tikzpicture}[shorten >=1pt,->,draw=black!50, node distance=\layersep]
    \tikzstyle{every pin edge}=[<-,shorten <=1pt]
    \tikzstyle{neuron}=[circle,fill=black!25,minimum size=17pt,inner sep=0pt]
    \tikzstyle{input neuron}=[neuron, fill=green!50];
    \tikzstyle{output neuron}=[neuron, fill=red!50];
    \tikzstyle{hidden neuron}=[neuron, fill=blue!50];
    \tikzstyle{black neuron}=[neuron, fill=black!80];
    \tikzstyle{annot} = [text width=4em, text centered]

    \foreach \name / \y in {1,...,4}
        \node[input neuron, pin=left:Input \#\y] (I-\name) at (0,-\y) {};

    \foreach \name / \y in {1,...,5}
        \path[yshift=0.5cm]
            node[hidden neuron] (H-\name) at (\layersep,-\y cm) {};

    \foreach \name / \y in {1,...,4}
            \node[input neuron] (Ho-\name) at (2*\layersep,-\y) {};

    \node[black neuron, right of=Ho-3] (B) at (2*\layersep,-2.5 cm) {};
    
    \node[output neuron,pin={[pin edge={->}]right:Output}, right of=B] (O) {};

    \foreach \source in {1,...,4}
        \foreach \dest in {1,...,5}
            \path (I-\source) edge (H-\dest);

    \foreach \source in {1,...,5}
        \foreach \dest in {1,...,4}
            \path (H-\source) edge (Ho-\dest);

    \foreach \source in {1,...,4}
        \path (Ho-\source) edge (B);
        
    \path (B) edge (O);

    \node[annot,above of=H-1, node distance=1cm] (hl) {Hidden layer};
    \node[annot,right of=hl] (h2) {New representation};
    \node[annot,left of=hl] {Input layer};
    \node[annot,right of=h2] (bb) {Black-box};
    \node[annot,right of=bb] {Output layer};
    
    \draw[draw=black, line width=1mm] (1.4,-5.0) rectangle ++(7.3,6.5);
\end{tikzpicture}
\caption{The idea}
\label{fig:idea}
\end{figure*}
